# Supplementary material for: Functional Stability of Discounted Markov Decision Processes Using Economic MPC Dissipativity Theory
Source: arXiv:2203.16989 source file (2022-03-31)
Supplement: Supplementary file 1 [file additional.tex]

%The paper is structured as follows. Section \ref{sec:PS} describes the problem setting and formulates MDPs in the density space. We introduce optimal value functional and optimal steady measure in this section. Section \ref{sec:stability} details the functional stability concept and FSDSD conditions for MDPs. In this section, we show that a closed-loop Markov chain is functional stable under the optimal policy if the associated MDP satisfies FSDSD conditions. Section \ref{sec:FA} a introduces functional approximator for the optimal action-value function, which delivers a valid storage function for rich enough parameterization. Section \ref{sec:Conc} delivers the conclusions.
%Section \ref{sec:NS} provides numerical simulation results, and  

For the discounted setting the stage cost \eqref{eq:TL} reads:
\begin{align}
  &L(\vect s,\vect a)=\\ &\left\{\begin{matrix}
 Q^\star(\vect s,\vect a)- V^\star(\vect f(\vect s,\vect a)) & \mathrm{If}\, \left|V^\star(\vect f(\vect s,\vect a))\right|<\infty \\ \infty
 & \mathrm{Otherwise}
\end{matrix}\right.\nonumber
\end{align}
then if there exists a storage function $\lambda$:
\begin{align}
    \lambda (\vect f(\vect s,\vect a)) - \lambda (\vect s) \leq -\rho(\|\vect s\|)+ Q^\star(\vect s,\vect a)- V^\star(\vect f(\vect s,\vect a))
\end{align}
then MPC is dissipative. If the model is same as the real system, then this condition is exactly the second condition of SDSD. Then we can write:
\begin{align}
 V^\star(\vect s)=-\lambda(\vect s)+\min_{\vect\pi}   V^\star(\hat{\vect s}_N)+\sum_{k=0}^{N-1} \bar L(\hat {\vect s}_k,\vect { \pi}\left(\hat {\vect s}_k\right)),\,\, \hat {\vect s}_0=\vect s,
\end{align}
where 
\begin{align}
    &\rho(\|\vect s\|)\leq \bar L(\vect s,\vect a)=:\\ &Q^\star(\vect s,\vect a)- V^\star(\vect f(\vect s,\vect a))+\lambda (\vect s)-\lambda (\vect f(\vect s,\vect a))\nonumber
\end{align}

\section{Functional Dissipativity \& Learning}
We won't have enough time to propose something ``solid", but some reflections to pave the way to what we could say soon would be meaningful. Here are a few thoughts:
\begin{itemize}
    \item We can make the argument for ``learning under the dissipativity constraints" rather than ``verifying the dissipativity constraints" (similar to other papers). In that context, we learn an MPC with a functional stage cost satisfying (6), where the storage function acts as an ``extra degree of freedom" to achieve Q-learning. We may have to admit that the undiscounted case (reverting to the original functional dissipativity) is easier to treat.
\item We could unpack a bit what Q-learning looks like in the functional case. Generally speaking it would be something of the kind:
\begin{align}
    \min_{\vect\theta}\, \mathbb E\left[Q_{\vect\theta}[\delta_{\vect s},\vect a] - Q^\star(\vect s,\vect a)\right]^2
\end{align}
where $\delta_{\vect s}$ is a Dirac measure taken at $\vect s$ and $\mathbb E$ is an expected value over the real state transitions and the exploration (we don't have much of a choice here). What does it imply? 
\item We could add the ``cost modification" story here for the functional case, and then argue that the functional MPC does not need to use a perfect model (and/or could even be deterministic). 
\end{itemize}

Next lemma states the monotonicity property of functional ${\Psi}_{\vect\theta}^{N}$ with respect to the horizon length $N$.
\begin{Lemma} Suppose that \eqref{eq:ter:assum} holds. Then:
\begin{align}\label{eq:mono}
    {\Psi}^{N+1}_{\vect\theta}[\rho_0]\leq {\Psi}^{N}_{\vect\theta}[\rho_0], \quad \forall N\in\mathbb{I}_{\geq 0}
\end{align}

\end{Lemma}
\begin{proof}
For $N=0$, from \eqref{eq:ter:assum}, we have:
\begin{align}
   V^1_{\vect\theta}[\rho_0]&=\min_{\vect\pi}{-\lambda_{\vect\theta}[\rho_0]+T_{\vect\theta}[\rho^{\vect\pi}_1]+\mathcal{L}_{\vect\theta}[\rho_0,\vect\pi]}\nonumber\\&\leq -\lambda_{\vect\theta}[\rho_0]+T_{\vect\theta}[\rho_0]:=V^0_{\vect\theta}[\rho_0]
\end{align}
where $\rho^{\vect\pi}_1\in\Xi_{\mathrm{f}}$. Suppose that for some $N\geq0$, \eqref{eq:mono} holds, then for $N+1$ we have:
\begin{align}\label{eq:pro1}
     V^{N+2}_{\vect\theta}[\rho_0]-&V^{N+1}_{\vect\theta}[\rho_0]= \mathcal{L}_{\vect\theta}[\rho_0,\vect\pi^{N+2}_{\vect\theta}]+V^{N+1}_{\vect\theta}[\rho^{\vect\pi^{N+2}_{\vect\theta}}_1]\nonumber\\&-\mathcal{L}_{\vect\theta}[\rho_0,\vect\pi^{N+1}_{\vect\theta}]-V^{N}_{\vect\theta}[\rho^{\vect\pi^{N+1}_{\vect\theta}}_1]
\end{align}
Then $\vect\pi^{N+1}_{\vect\theta}$ may not be optimal for the value function $V^{N+2}_{\vect\theta}[\rho_0]$ and \eqref{eq:pro1} reads as:
\begin{align}
    V^{N+2}_{\vect\theta}[\rho_0]&-V^{N+1}_{\vect\theta}[\rho_0]\leq \mathcal{L}_{\vect\theta}[\rho_0,\vect\pi^{N+1}_{\vect\theta}]+V^{N+1}_{\vect\theta}[\rho^{\vect\pi^{N+1}_{\vect\theta}}_1]\nonumber\\&-\mathcal{L}_{\vect\theta}[\rho_0,\vect\pi^{N+1}_{\vect\theta}]+V^{N}_{\vect\theta}[\rho^{\vect\pi^{N+1}_{\vect\theta}}_1]\leq 0
\end{align}
then by induction \eqref{eq:mono} holds $\forall N\in\mathbb{I}_{\geq 0}$.
\end{proof}

We next assume that the stage cost ${\mathcal{L}_{\vect\theta}}[\rho_0,\vect\pi]$, the terminal cost $T_{\vect\theta}$ and the terminal set $\Xi_{\mathrm{f}}$ satisfy the stabilizing conditions.
\begin{Assumption}\label{assum:LT}We assume that the stage cost satisfies:

and there exists a terminal policy $\vect\pi_{\mathrm{f}}$ such that the terminal cost $T_{\vect\theta}$ satisfies the following conditions, $\forall \rho_0\in\Xi_{\mathrm{f}}$:
\begin{subequations}
\begin{align}\label{eq:ter:assum}
    T_{\vect\theta}[\rho^{\vect\pi_{\mathrm{f}}}_{1}]-T_{\vect\theta}[\rho_{0}]&\leq-{\mathcal{L}_{\vect\theta}}[\rho_0,\vect\pi_{\mathrm{f}}]\\
\label{eq:ter2:assum}
    T_{\vect\theta}[\rho_0] &\geq 0\,\,,  
\end{align}
\end{subequations}
\end{Assumption}
Note that this assumption is a standard assumption for tracking MPC in order to show the closed-loop stability under the optimal policy resulting from the MPC-scheme. The terminal cost assumption can be satisfied using a generic non-negative functional approximator and designing a proper terminal set that contains the optimal steady-state measure $\rho^\star$. The stage cost assumption can be satisfied using constrained steps in the learning algorithm or providing a positive functional by construction. The details of these methods for deterministic systems can be found in \cite{Arash2021verification}. However, a detailed discussion on functional space is out of our scope.
